# Supplementary material for: Interactive Humanoid: Online Full-Body Motion Reaction Synthesis with Social Affordance Canonicalization and Forecasting
Source: arXiv:2312.08983 source file (2024-02-05)
Supplement: Supplementary file 1 [file X_suppl.tex]

\clearpage
\setcounter{page}{1}
\maketitlesupplementary
% 1. 拥抱
% 2. 握手
% 3. 拍手鼓掌
% 4. 摇手臂
% 5. 互相搀扶
% 6. 拿出手机分享内容
% 7. 同时跳舞   
% 8. 一人指出方向，另一人跟随
% 9. 一人比划相机，另一人摆出姿势
% 10. 一起下棋
% 11. 一人举手示意停车，另一人扮演交通警察
% 12. 互相做出"加油"手势
% 13. 一人模仿跳舞，另一人击鼓伴奏
% 14. Say hi
% 15. 互相作出欢呼的手势
% 16. 互相比划谁更高
% 17. 捶背
% 18. 一人模仿坐下，另一人帮助拉椅子
% 19. 一人模仿开门，另一人模仿进门
% 20. 互相模仿打拳的动作
% 21. 互相模仿跳绳的动作
% 22. 一人模仿吹泡泡，另一人模仿追逐
% 23. 一人模仿起身，另一人模仿扶持
% 24. 相互扔东西
% 25. 一人模仿打太极拳，另一人模仿跟随
% 26. 互相模仿摆动腰部的动作
% 27. 一起拉伸
% 28. 互相模仿击掌的动作
% 29. 合掌鞠躬
% 30. 漫步and 走秀
% 31. 互相搭肩
% 32. 一人模仿为另一人系领带
% 33. 一人模仿为另一人系腰带
% 34. 一人模仿为另一人拉上拉链
% 35. 一人模仿为另一人整理袖口
% 36. 一人模仿为另一人捡起物品
% 37. 抛东西
% 38. 一人模仿为另一人挥动扇子
% 39. 一人模仿为另一人递饮料
% 40. 拜拜
